# Supplementary material for: Neural Fields in Visual Computing and Beyond
Source: arXiv:2111.11426 source file (2022-04-05)
Supplement: Supplementary file 1 [file appendix_all_works.tex]

\newpage
\onecolumn
\begin{longtable}[c]{|p{2.2cm}|p{1.7cm}|p{0.04cm}|p{0.04cm}|p{0.04cm}|p{0.04cm}|p{0.04cm}|p{0.04cm}|p{0.04cm}|p{0.04cm}|p{0.04cm}|p{0.04cm}|p{0.04cm}|p{0.04cm}|p{0.04cm}|p{0.04cm}|p{0.04cm}|p{0.04cm}|p{0.04cm}|p{0.04cm}|p{0.04cm}|p{0.04cm}|p{0.04cm}|p{0.04cm}|p{0.04cm}|p{0.04cm}|p{0.04cm}|p{0.04cm}|p{0.04cm}|p{0.04cm}|}
\caption{Tabulated keywords for all neural fields papers. Keyword lookup: 0: Speed (Training), 1: Speed (Rendering), 2: Sparse Reconstruction, 3: Dynamic, 4: Human (Body), 5: Human (Head), 6: Robotics, 7: Image, 8: Camera Parameter Estimation, 9: Material/Lighting Estimation, 10: Editable, 11: Compression, 12: Alternative Imaging, 13: Science \& Engineering, 14: Fundamentals, 15: Generative Models, 16: Generalization, 17: Global Conditioning, 18: Local Conditioning, 19: Image-based Rendering, 20: Hypernetwork/Meta-learning, 21: Hybrid Geometry Parameterization, 22: Voxel Grid, 23: Object-Centric, 24: Sampling, 25: Supervision by Gradient (PDE), 26: Coarse-to-Fine, 27: Coordinate Re-mapping.}\\

\toprule
\multicolumn{1}{|c|}{\textbf{Title}} & \multicolumn{1}{|c|}{\textbf{Citation}} & \multicolumn{1}{|c|}{0} & \multicolumn{1}{|c|}{1} & \multicolumn{1}{|c|}{2} & \multicolumn{1}{|c|}{3} & \multicolumn{1}{|c|}{4} & \multicolumn{1}{|c|}{5} & \multicolumn{1}{|c|}{6} & \multicolumn{1}{|c|}{7} & \multicolumn{1}{|c|}{8} & \multicolumn{1}{|c|}{9} & \multicolumn{1}{|c|}{10} & \multicolumn{1}{|c|}{11} & \multicolumn{1}{|c|}{12} & \multicolumn{1}{|c|}{13} & \multicolumn{1}{|c|}{14} & \multicolumn{1}{|c|}{15} & \multicolumn{1}{|c|}{16} & \multicolumn{1}{|c|}{17} & \multicolumn{1}{|c|}{18} & \multicolumn{1}{|c|}{19} & \multicolumn{1}{|c|}{20} & \multicolumn{1}{|c|}{21} & \multicolumn{1}{|c|}{22} & \multicolumn{1}{|c|}{23} & \multicolumn{1}{|c|}{24} & \multicolumn{1}{|c|}{25} & \multicolumn{1}{|c|}{26} & \multicolumn{1}{|c|}{27}
\midrule
\endfirsthead

\multicolumn{30}{c}%
{{Tabulated keywords for all neural fields papers. Keyword lookup: 0: Speed (Training), 1: Speed (Rendering), 2: Sparse Reconstruction, 3: Dynamic, 4: Human (Body), 5: Human (Head), 6: Robotics, 7: Image, 8: Camera Parameter Estimation, 9: Material/Lighting Estimation, 10: Editable, 11: Compression, 12: Alternative Imaging, 13: Science \& Engineering, 14: Fundamentals, 15: Generative Models, 16: Generalization, 17: Global Conditioning, 18: Local Conditioning, 19: Image-based Rendering, 20: Hypernetwork/Meta-learning, 21: Hybrid Geometry Parameterization, 22: Voxel Grid, 23: Object-Centric, 24: Sampling, 25: Supervision by Gradient (PDE), 26: Coarse-to-Fine, 27: Coordinate Re-mapping.}} \\
\toprule
\multicolumn{1}{|c|}{\textbf{Title}} & \multicolumn{1}{|c|}{\textbf{Citation}} & \multicolumn{1}{|c|}{0} & \multicolumn{1}{|c|}{1} & \multicolumn{1}{|c|}{2} & \multicolumn{1}{|c|}{3} & \multicolumn{1}{|c|}{4} & \multicolumn{1}{|c|}{5} & \multicolumn{1}{|c|}{6} & \multicolumn{1}{|c|}{7} & \multicolumn{1}{|c|}{8} & \multicolumn{1}{|c|}{9} & \multicolumn{1}{|c|}{10} & \multicolumn{1}{|c|}{11} & \multicolumn{1}{|c|}{12} & \multicolumn{1}{|c|}{13} & \multicolumn{1}{|c|}{14} & \multicolumn{1}{|c|}{15} & \multicolumn{1}{|c|}{16} & \multicolumn{1}{|c|}{17} & \multicolumn{1}{|c|}{18} & \multicolumn{1}{|c|}{19} & \multicolumn{1}{|c|}{20} & \multicolumn{1}{|c|}{21} & \multicolumn{1}{|c|}{22} & \multicolumn{1}{|c|}{23} & \multicolumn{1}{|c|}{24} & \multicolumn{1}{|c|}{25} & \multicolumn{1}{|c|}{26} & \multicolumn{1}{|c|}{27}
\midrule

\midrule 
\multicolumn{30}{|r|}{Continued on next page} \\ 
\midrule
\endfoot
StyleNeRF & \cite{anonymous2022stylenerf} &   &   &   &   &   &   &   &   &   &   &   &   &   &   &   &   &   &   &   &   &   &   &   &   &   &   &   &  \\
TöRF & \cite{attal2021torf} &   &   &   & \checkmark &   &   &   &   &   &   &   &   & \checkmark &   &   &   &   & \checkmark & \checkmark &   &   &   &   &   &   &   &   &  \\
Neural Knitworks & \cite{czerkawski2021neuralknitworks} &   &   &   &   &   &   &   & \checkmark &   &   &   &   &   &   &   & \checkmark &   &   &   &   &   &   &   &   &   &   &   &  \\
ImplicitVol & \cite{yeung2021implicitvol} &   &   &   &   &   &   &   &   &   &   &   &   & \checkmark & \checkmark &   &   &   &   &   &   &   &   &   &   &   &   &   &  \\
HALO & \cite{karunratanakul2021halo} &   &   &   &   &   &   &   &   &   &   &   &   &   &   &   &   &   &   &   &   &   &   &   &   &   &   &   & \checkmark\\
Kasten et al. & \cite{kasten2021layered} &   &   &   & \checkmark &   &   &   & \checkmark &   &   & \checkmark &   &   &   &   &   &   &   &   &   &   &   &   &   &   &   &   &  \\
Juhl et al. & \cite{juhl2021implicit} &   &   &   &   & \checkmark & \checkmark &   &   &   &   &   &   &   & \checkmark &   &   &   & \checkmark &   &   &   &   &   &   &   &   &   &  \\
Hu et al. & \cite{hu2021when} &   &   &   &   &   &   &   &   &   &   &   &   &   & \checkmark &   &   &   &   &   &   &   &   &   &   &   &   &   &  \\
Neural Cameras & \cite{mandl2021neuralcameras} &   &   &   &   &   &   &   &   & \checkmark &   &   &   &   &   &   &   &   &   &   &   &   &   &   &   &   &   &   &  \\
ObjectFolder & \cite{gao2021objectfolder} &   &   &   &   &   &   & \checkmark &   &   &   &   & \checkmark &   & \checkmark &   &   &   &   &   &   &   &   &   &   &   &   &   &  \\
Neural Human Performer & \cite{kwon2021neuralhumanperformer} &   &   &   & \checkmark & \checkmark &   &   &   &   &   &   &   &   &   &   &   & \checkmark &   & \checkmark &   &   &   &   &   &   &   &   &  \\
MDIF & \cite{chen2021mdif} &   &   &   &   &   &   &   &   &   &   &   &   &   &   &   &   &   &   & \checkmark &   &   &   & \checkmark &   &   &   & \checkmark &  \\
NEAT & \cite{chitta2021neat} &   &   &   & \checkmark &   &   &   &   &   &   &   &   &   & \checkmark &   &   &   &   &   &   &   &   &   &   &   &   &   &  \\
S-NeRF & \cite{shen2021snerf} &   &   &   &   &   &   &   &   &   &   &   &   &   &   & \checkmark &   &   &   &   &   &   &   &   &   &   &   &   &  \\
Yang et al. & \cite{yang2021learning} &   &   &   &   &   &   &   &   &   &   & \checkmark &   &   &   &   &   &   & \checkmark & \checkmark &   &   &   & \checkmark & \checkmark &   &   &   &  \\
CodeNeRF & \cite{jang2021codenerf} &   &   &   &   &   &   &   &   &   &   & \checkmark &   &   &   &   &   & \checkmark & \checkmark &   &   &   &   &   &   &   &   &   &  \\
NerfingMVS & \cite{wei2021nerfingmvs} &   &   &   &   &   &   &   &   &   &   &   &   &   &   &   &   &   &   & \checkmark &   &   &   &   &   & \checkmark &   &   &  \\
IntraTomo & \cite{zang2021intratomo} &   &   &   &   &   &   &   &   &   &   &   &   & \checkmark & \checkmark &   &   &   &   &   &   &   &   &   &   &   &   &   &  \\
Huang et al. & \cite{huang2021a} &   &   &   &   &   &   &   &   &   &   &   &   &   & \checkmark & \checkmark &   &   &   &   &   &   &   &   &   &   & \checkmark &   &  \\
Benbarka et al. & \cite{benbarka2021seeing} &   &   &   &   &   &   &   & \checkmark &   &   &   &   &   &   & \checkmark &   &   &   &   &   &   &   &   &   &   &   & \checkmark &  \\
CO3D & \cite{reizenstein2021co3d} &   &   & \checkmark &   &   &   &   &   &   &   &   &   &   &   &   &   & \checkmark &   & \checkmark &   &   &   &   &   &   &   &   &  \\
Jeong et al. & \cite{jeong2021selfcalibrating} &   &   &   &   &   &   &   &   & \checkmark &   &   &   &   &   &   &   &   &   &   &   &   &   &   &   &   &   & \checkmark &  \\
NeRP & \cite{shen2021nerp} &   &   &   &   &   &   &   &   &   &   &   &   & \checkmark & \checkmark &   &   & \checkmark &   &   &   &   &   &   &   &   &   &   &  \\
imGHUM & \cite{alldieck2021imghum} &   &   &   &   & \checkmark &   &   &   &   &   &   &   &   &   &   &   &   &   &   &   &   &   &   &   &   &   &   &  \\
Reed et al. & \cite{reed2021implicit} &   &   &   &   &   &   &   &   &   &   &   &   & \checkmark & \checkmark &   &   &   &   &   &   &   &   &   &   &   &   &   &  \\
Zhang et al. & \cite{zhang2021learning} &   &   &   &   &   &   &   &   &   &   &   &   &   &   &   &   &   &   &   &   &   &   &   &   &   &   &   &  \\
Wu et al. & \cite{wu2021learning} &   &   &   &   &   &   &   &   &   &   &   &   &   &   & \checkmark &   &   &   &   &   &   &   &   &   &   &   &   &  \\
Neural-GIF & \cite{tiwari2021neuralgif} &   &   &   &   & \checkmark &   &   &   &   &   &   &   &   &   &   &   &   &   &   &   &   &   &   &   &   &   &   & \checkmark\\
Atzmon et al. & \cite{atzmon2021augmenting} &   &   &   & \checkmark & \checkmark &   &   &   &   &   &   &   &   &   &   &   &   &   &   &   &   &   &   &   &   &   &   & \checkmark\\
ARCH++ & \cite{he2021arch++} &   &   & \checkmark &   & \checkmark &   &   &   &   &   & \checkmark &   &   &   &   &   &   &   & \checkmark &   &   &   & \checkmark &   &   &   &   &  \\
Li et al. & \cite{li2021unsupervised} &   &   &   &   &   &   &   & \checkmark &   &   &   &   & \checkmark &   &   &   &   &   &   &   &   &   &   &   &   &   &   &  \\
Yan et al. & \cite{yan2021continual} &   &   &   &   &   &   & \checkmark &   &   &   &   &   &   &   &   &   &   & \checkmark &   &   &   &   &   &   &   &   &   &  \\
SIDER & \cite{chatziagapi2021sider} &   &   & \checkmark &   &   & \checkmark &   &   &   &   &   &   &   &   &   &   & \checkmark &   &   &   &   &   &   &   &   &   & \checkmark &  \\
FLAME-in-NeRF & \cite{athar2021flameinnerf} &   &   &   & \checkmark &   & \checkmark &   &   &   &   & \checkmark &   &   &   &   &   & \checkmark & \checkmark &   &   &   &   &   &   &   &   & \checkmark & \checkmark\\
Khademi et al. & \cite{khademi2021view} &   &   &   &   &   &   &   &   &   &   &   &   &   &   &   &   &   &   &   &   &   &   &   &   & \checkmark &   &   &  \\
Nam et al. & \cite{nam2021neural} &   &   &   & \checkmark &   &   &   & \checkmark &   &   &   &   &   &   &   &   &   &   &   &   &   &   &   &   &   &   &   & \checkmark\\
H3D-Net & \cite{ramon2021h3dnet} &   &   & \checkmark &   &   & \checkmark &   &   &   &   &   &   &   &   &   &   &   & \checkmark &   &   &   &   &   &   &   &   &   &  \\
NeLF & \cite{sun2021nelf} &   &   &   &   &   & \checkmark &   &   &   & \checkmark &   &   &   &   &   &   &   &   & \checkmark &   &   &   &   &   &   &   &   &  \\
Zobeidi et al. & \cite{zobeidi2021a} &   &   &   &   &   &   &   &   &   &   &   &   &   &   &   &   &   &   &   &   &   &   &   &   &   &   &   &  \\
GFNN & \cite{dehesa2021gfnn} &   &   &   &   &   &   &   &   &   &   &   &   &   & \checkmark & \checkmark &   &   &   &   &   &   &   &   &   &   &   &   &  \\
uORF & \cite{yu2021uorf} &   &   &   &   &   &   &   &   &   &   & \checkmark &   &   &   &   &   & \checkmark &   & \checkmark &   &   &   &   & \checkmark &   &   &   &  \\
FBPINNs & \cite{moseley2021fbpinns} &   &   &   &   &   &   &   &   &   &   &   &   &   & \checkmark &   &   &   &   &   &   &   &   &   &   &   &   &   &  \\
Pan et al. & \cite{pan2021adaptive} &   &   &   &   &   &   &   &   &   &   &   &   & \checkmark & \checkmark &   &   &   &   &   &   &   &   &   &   &   &   &   &  \\
Li et al. & \cite{li20213d} &   &   &   &   &   &   & \checkmark &   &   &   &   &   &   & \checkmark &   &   &   &   &   &   &   &   &   &   &   &   &   &  \\
Zheng et al. & \cite{zheng2021rethinking} &   &   &   &   &   &   &   &   &   &   &   &   &   &   & \checkmark &   &   &   &   &   &   &   &   &   &   &   &   &  \\
DS-NeRF & \cite{deng2021dsnerf} & \checkmark &   & \checkmark &   &   &   &   &   &   &   &   &   &   &   &   &   &   &   &   &   &   &   &   &   &   &   &   &  \\
IREM & \cite{wu2021irem} &   &   &   &   &   &   &   &   &   &   &   &   &   &   &   &   &   &   &   &   &   &   &   &   &   &   &   &  \\
MetaNLR++ & \cite{bergman2021metanlr++} & \checkmark & \checkmark &   &   &   &   &   & \checkmark &   &   &   &   &   &   &   &   & \checkmark &   & \checkmark & \checkmark & \checkmark &   &   &   &   &   &   &  \\
Chen et al. & \cite{chen2021animatable} &   &   &   & \checkmark & \checkmark &   &   &   &   &   &   &   &   &   &   &   &   &   &   &   &   &   &   &   &   &   &   &  \\

\vspace{-0.25cm}
\end{longtable}
