# Supplementary material for: Neural Fields in Visual Computing and Beyond
Source: arXiv:2111.11426 source file (2022-04-05)
Supplement: Supplementary file 2 [file common_loss_in_recon.tex]

Common Loss Functions in 3D Reconstruction


%% YIHENG NOTE
% Geometry sparsity loss (useful for volume density)
% - To reconstruct hard surfaces, one can use the empty space loss and penalize volume density betwen the camera and object surface \cite{xian2020videonerf} $L=\int_{d_near}^{d_surface}{\sigma(x(t))} dt
% - Alternative
%% END YIHENG
