# Supplementary material for: Neural Fields in Visual Computing and Beyond
Source: arXiv:2111.11426 source file (2022-04-05)
Supplement: Supplementary file 3 [file off_the_shelf.tex]

Off-the-shelf methods used in neural fields:
- COLMAP
- SMPL
- MONOCULAR DEPTH ESTIMATION Networks
- RAFT
- 3DMM
